# Supplementary material for: Accelerating Image Super-Resolution Networks with Pixel-Level Classification
Source: arXiv:2407.21448 source file (2024-07-31)
Supplement: Supplementary file 1 [file fig_failure_case.tex]

% % Test2K

\begin{figure}[]
\centering
\tiny
\begin{tabular}
{@{}m{0.03\linewidth}@{\hskip2pt}m{0.24\linewidth}@{\hskip2pt}m{0.14\linewidth}@{\hskip2pt}m{0.14\linewidth}@{\hskip2pt}m{0.14\linewidth}@{\hskip2pt}m{0.14\linewidth}@{\hskip2pt}m{0.14\linewidth}@{}}

&
\small\centering{Classification (Ours)} &
\small\centering{ClassSR} &
\small\centering{ARM} &
\small\centering{Ours} &
\small\centering{Backbone} &
\small\centering{GT} \tabularnewline
\midrule

%5
\multirow{3}{*}[-6em]{\begin{subfigure}[m]{\linewidth}\caption{}\label{fig:visual_comparisons_a}\end{subfigure}} &
\multirow{3}{*}[-4em]{\includegraphics[width=\linewidth]{appendix/assets/fig_comparisons1/Urban100_060_004_y256_x128_Box.jpg}} &
\centering{22.42dB 40.8G(88\%)} &
\centering{22.49dB 40.0G(87\%)} &
\centering{22.64dB 32.6G(70\%)} &
\centering{22.61dB 46.3G(100\%)} &
\centering{} \tabularnewline
&
&
\includegraphics[width=\linewidth]{appendix/assets/fig_comparisons1/Urban100_060_004_y256_x128_ClassSR} &
\includegraphics[width=\linewidth]{appendix/assets/fig_comparisons1/Urban100_060_004_y256_x128_ARM} &
\includegraphics[width=\linewidth]{appendix/assets/fig_comparisons1/Urban100_060_004_y256_x128_Ours} &
\includegraphics[width=\linewidth]{appendix/assets/fig_comparisons1/Urban100_060_004_y256_x128_CARN} &
\includegraphics[width=\linewidth]{appendix/assets/fig_comparisons1/Urban100_060_004_y256_x128_GT} \tabularnewline
&
&
\includegraphics[width=\linewidth]{appendix/assets/fig_comparisons1/Urban100_060_004_y256_x128_ClassSR_Colored} &
\includegraphics[width=\linewidth]{appendix/assets/fig_comparisons1/Urban100_060_004_y256_x128_ARM_Colored} &
\includegraphics[width=\linewidth]{appendix/assets/fig_comparisons1/Urban100_060_004_y256_x128_Ours_Colored} &
&
\tabularnewline
\midrule

%5
\multirow{3}{*}[-6em]{\begin{subfigure}[m]{\linewidth}\caption{}\label{fig:visual_comparisons_a}\end{subfigure}} &
\multirow{3}{*}[0.2em]{\hspace{1em}\includegraphics[width=0.8\linewidth]{appendix/assets/fig_comparisons1/Test2K_036_000_y384_x000_Box.jpg}} &
\centering{20.80dB 111.5G(93\%)} &
\centering{20.75dB 105.0G(87\%)} &
\centering{20.78dB 78.6G(65\%)} &
\centering{20.82dB 120.3G(100\%)} &
\centering{} \tabularnewline
&
&
\includegraphics[width=\linewidth]{appendix/assets/fig_comparisons1/Test2K_036_000_y384_x000_ClassSR} &
\includegraphics[width=\linewidth]{appendix/assets/fig_comparisons1/Test2K_036_000_y384_x000_ARM} &
\includegraphics[width=\linewidth]{appendix/assets/fig_comparisons1/Test2K_036_000_y384_x000_Ours} &
\includegraphics[width=\linewidth]{appendix/assets/fig_comparisons1/Test2K_036_000_y384_x000_CARN} &
\includegraphics[width=\linewidth]{appendix/assets/fig_comparisons1/Test2K_036_000_y384_x000_GT} \tabularnewline
&
&
\includegraphics[width=\linewidth]{appendix/assets/fig_comparisons1/Test2K_036_000_y384_x000_ClassSR_Colored} &
\includegraphics[width=\linewidth]{appendix/assets/fig_comparisons1/Test2K_036_000_y384_x000_ARM_Colored} &
\includegraphics[width=\linewidth]{appendix/assets/fig_comparisons1/Test2K_036_000_y384_x000_Ours_Colored} &
&
\tabularnewline

\end{tabular}
\caption{
Failure case? limitation? classifier failed to accurately work on highly textured region, assigning those pixels to the light upsampler.
}
\label{fig:failure_case}
\end{figure}
